# Supplementary material for: Pistis-RAG: Enhancing Retrieval-Augmented Generation with Human Feedback
Source: arXiv:2407.00072 source file (2024-10-31)
Supplement: Supplementary file 1 [file appendix.tex]

\section*{Appendix}\label{sec:appendix}
The value of this approach lies in its ability to integrate with other methods within a content-centric framework, enhancing the system's end-to-end performance while minimizing disruption. From the practical perspective of content-centricity, there are many plugins that can be added as long as the business can balance latency and accuracy. The figure illustrates our complete system.

Content-centric architecture not only identifies issues but also extends the system's capabilities by adding more plugins, such as re-ranking, reasoning, and aggregating.

\begin{figure*}
    \centering
    \includegraphics[width=\linewidth]{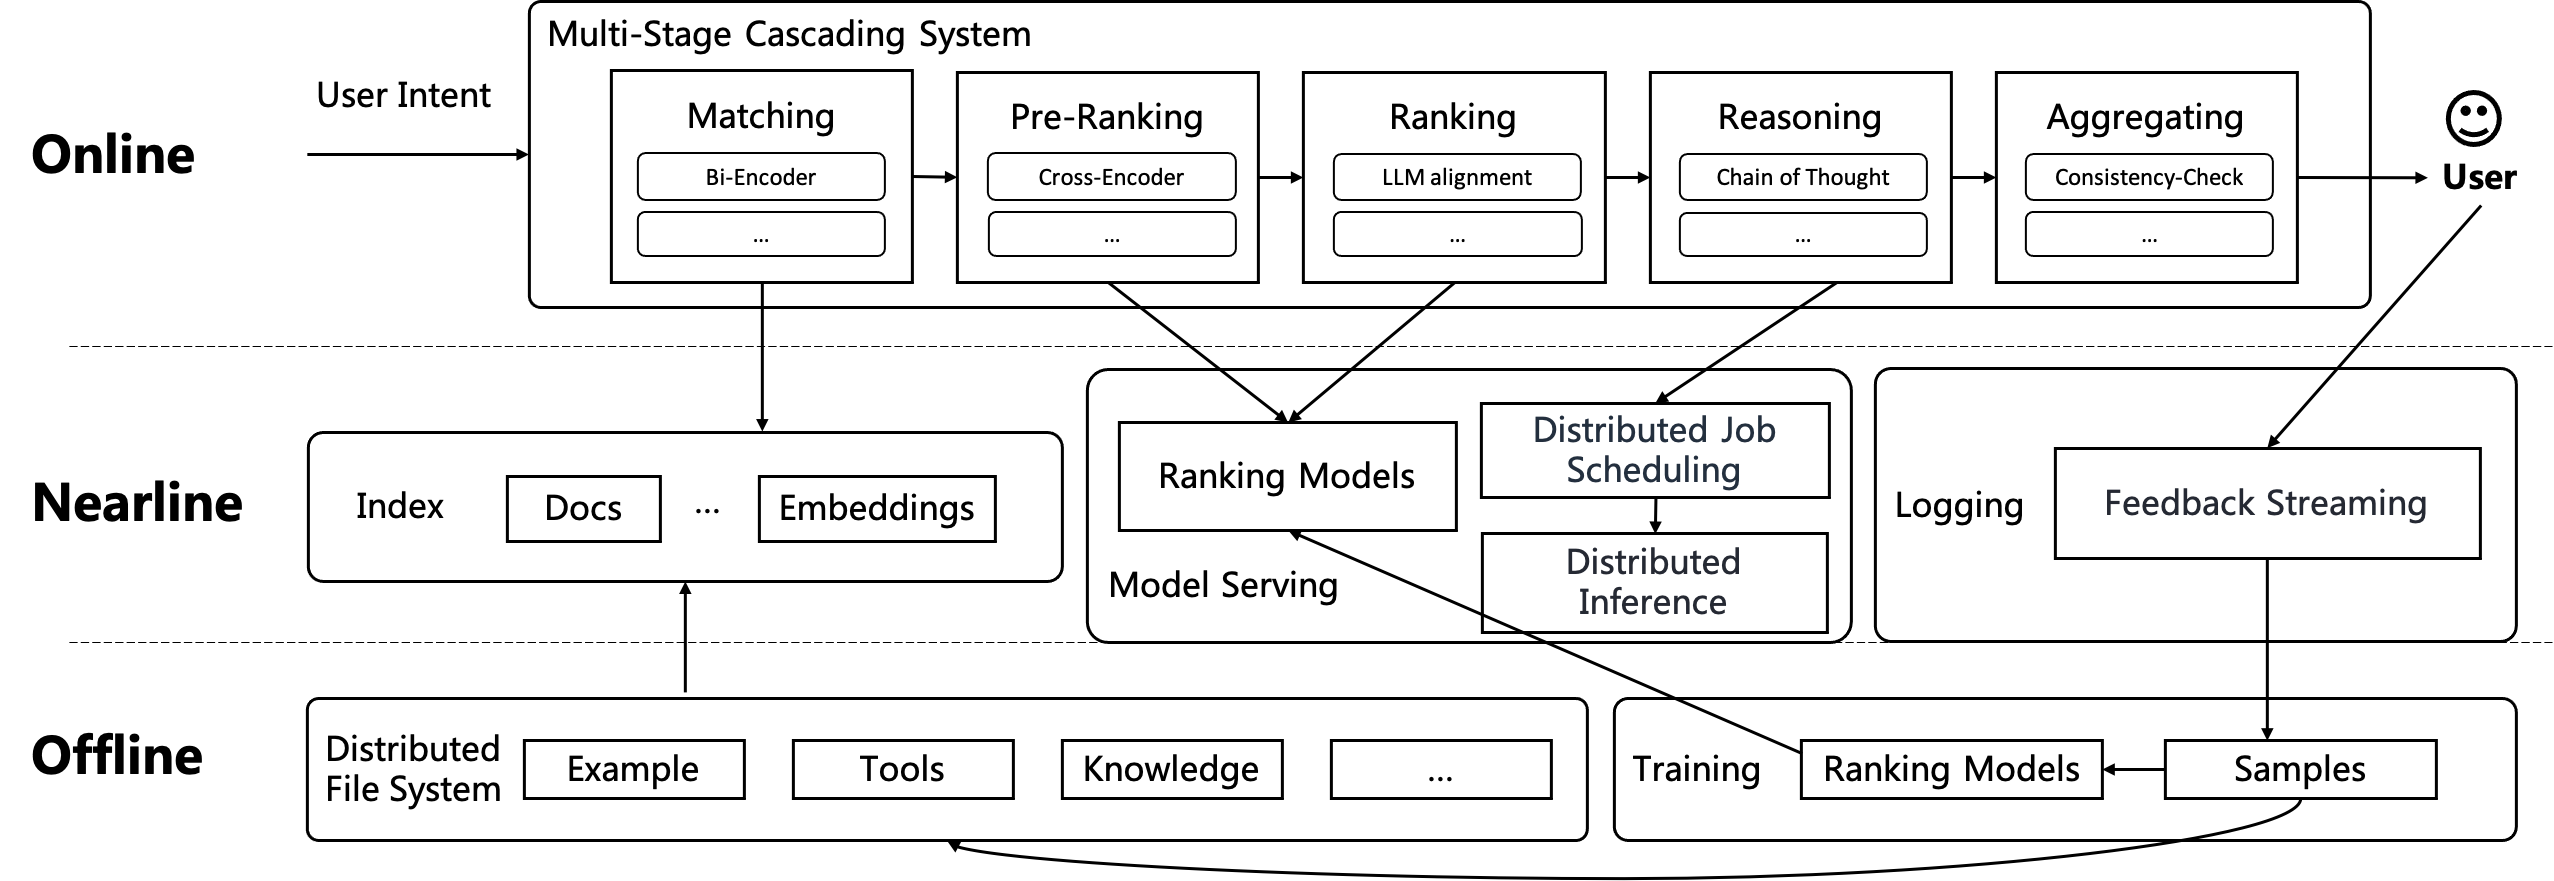}
    \caption[Pistis-RAG Framework]{Pistis-RAG Framework is designed to optimize information retrieval and response generation for LLMs. It is a comprehensive solution for complex queries and contextually relevant responses.}
    % \Description{Diagram of the Pistis-RAG Framework, detailing its five stages: Matching, Ranking, Reranking, Reasoning, and Aggregating. The framework optimizes information retrieval and response generation for LLMs using advanced techniques like Cross-Encoder methods and Concurrent Chain-of-Thought generation.}
    \label{fig:enter-label}
\end{figure*}

\begin{table*}[h]
\caption{Overview of Pistis-RAG Framework Stages and Industry Enhancements}
\label{tab:Pistis-RAG}
\begin{center}
\begin{tabular}{|>{\centering\arraybackslash}m{2.5cm}|>{\centering\arraybackslash}m{1.5cm}|>{\centering\arraybackslash}m{3cm}|>{\centering\arraybackslash}m{3cm}|>{\centering\arraybackslash}m{3cm}|>{\centering\arraybackslash}m{3cm}|}
\hline
\textbf{Stage} & \textbf{Item Size} & \textbf{Function} & \textbf{Techniques} & \textbf{Challenges} & \textbf{Industry} \\ \hline
Matching & Tens of Thousands & Retrieve relevant documents quickly & TF-IDF, BM25, Bi-Encoder & Ensuring relevance with mixed methods & Integration with external search engines \\ \hline
Pre-ranking & Hundreds & Reduce workload for the ranking stage & Cross-Encoder & Balancing accuracy and relevance & Auto-scaling and failover mechanisms \\ \hline
Ranking & Tens & Rank based on human preferences & Listwise LTR with listwide labels & Learning from listwide labels & Auto-scaling and failover mechanisms \\ \hline
Re-ranking & Few & Refine ranking based on additional criteria & Pointwise ranking algorithms & Meeting user-specific criteria & Ensuring credibility of generated content \\ \hline
Reasoning & - & Generate reasoned outputs through LLM inference & Multi-Path reasoning & Maintaining coherence in responses & Speculative decoding for performance \\ \hline
Aggregating & - & Synthesize coherent responses from reasoning & Consistency checks & Ensuring credibility and readability & Citations, Markdown formatting, content safety \\ \hline
\end{tabular}
\end{center}
\end{table*}

\subsection{Content-Centric System Architecture}
% 这个方法的价值在于在 content-centric 的框架中可以和其他方法配合使用，提高系统的端到端效果，并且对系统的侵扰很小。
% 从 content-centric 实用性的角度，我们还有很多可以增加的 plugin，只要在业务中可以平和 latency 和 accuracy 的关系，就可以使用。图中介绍了我们完整的系统。
% content-centric 不仅识别出了问题，而且为系统增加了更多扩展。

The Full Pistis-RAG Framework is designed to optimize online content-centric services. It consists of five stages: Matching, Pre-Ranking, Ranking, Reasoning, and Aggregating. In the Matching stage, retrieval algorithms select relevant documents from repositories. Semantic analysis in the Pre-Ranking stage refines document scores based on query relevance. Ranking aligns document rankings with LLM preferences for coherent responses. Reasoning enhances response diversity by exploring multiple sequences. The Aggregation stage synthesizes responses for coherence. Pistis-RAG employs advanced techniques, such as Cross-Encoder methods and Concurrent Chain-of-Thought generation, to enhance performance and response quality. It is a comprehensive solution for complex queries and contextually relevant responses.

The Pistis-RAG system architecture includes four core components: Matching, Ranking, Reasoning, and Aggregating Services, each meticulously designed to handle specific segments of the query-response cycle efficiently.

\subsubsection*{\textbf{Matching Service}}

The Matching Service is central to the user interaction process, responsible for understanding user intent and quickly retrieving the most relevant information. To achieve this, the Matching Service uses a sophisticated blend of IR techniques, optimizing latency for large-scale online retrieval.

The Matching Service employs various data structures to enhance information retrieval based on the specific technique:

\begin{itemize}
\item Vector Storage: This structure is essential for embedding-based retrieval approaches like ANN. It efficiently stores document representations as vectors, allowing for fast similarity comparisons with the user's query vector. For example, the Matching Service represents documents as vectors in a high-dimensional space, enabling quick identification of those semantically similar to the user's query.
\item Inverted Index: A key data structure for keyword-based retrieval, allowing rapid identification of documents containing specific keywords in the user's query. For example, when a user searches for a term, the inverted index directs the Matching Service to documents containing that term efficiently.
\end{itemize}

In-memory K-V Cache also plays a critical role in stateful services. It can be used for:

\begin{itemize}
\item Maintaining User Conversation Sessions: Storing the context of a user's ongoing conversation allows for a more coherent and personalized experience. For example, the Matching Service uses the K-V cache to remember the user's previous queries and interactions, enabling more tailored responses.
\item User Prompt-Answer Pair Cache: Storing previously accessed responses to common questions or prompts can significantly enhance response times. Additionally, it serves as an effective few-shot example for RAG. For instance, when a user poses a recurring question, the Matching Service saves the corresponding answer in the key-value cache, eliminating the need for a new search each time.
\item User-Relevant Session History: By storing high-quality content relevant to the user's past interactions, the Matching Service prioritizes its retrieval for future queries, improving the user experience. For example, if a user has shown interest in a particular topic, the Matching Service prioritizes content related to that topic when responding to future queries.
\end{itemize}

In large-scale industrial settings, the Matching Service might also integrate with external search engines to access a vast corpus of information. However, this approach typically increases latency due to network communication overhead.

The choice of retrieval technique and data structure depends on the specific requirements of the application. For instance, if higher accuracy is desired, ANN or inverted index and BM25 and TF-IDF methods can be used together. It is important to carefully consider the trade-offs between speed and accuracy when selecting the appropriate techniques.

Notably, it is important to acknowledge that the Matching Service has its limitations. For example, it may struggle with handling ambiguous or complex queries that require.

\subsubsection*{\textbf{Ranking Service}}

The Ranking Service optimizes the information retrieval process by prioritizing items that are most relevant to the user's intent. This prioritization considers both the retrieved items and the user's intent representation.

The Ranking Service employs several techniques to achieve this, organized into key stages:

\begin{enumerate}
\item \textbf{Stage 1: Pre-Ranking}
The Pre-Ranking stage serves as an initial filtering mechanism to streamline the subsequent ranking process. The principles have been detailed in the main text, so they are not repeated in the appendix. Some industry-specific configurations are listed in Table \ref{tab:Pistis-RAG}.

\item \textbf{Stage 2: Ranking}
The Ranking stage refines the relevance assessment process by scoring each item in the pre-ranked subset. The principles have been detailed in the main text, so they are not repeated in the appendix. Some industry-specific configurations are listed in Table \ref{tab:Pistis-RAG}.

\item \textbf{Stage 3: Re-Ranking}
The Re-Ranking phase, while optional, plays a crucial role in contexts such as official document composition or critical decision-making scenarios. Some industry-specific configurations are listed in the in Table \ref{tab:Pistis-RAG}.
\end{enumerate}

By prioritizing accuracy and relevance, the Ranking Service enhances the clarity, comprehensiveness, and effectiveness of the information retrieval process, providing users with a more valuable and trustworthy experience.

\subsubsection*{\textbf{Reasoning Service}}

The Reasoning Service enhances reasoning through parallel inference and expert routing. It leverages an advanced Chain of Thought~\cite{wei2022chain} to execute parallel inference across LLMs, generating diverse results for subsequent aggregation. This service takes prompts and retrieved information as input, producing a series of reasoned outputs. By harnessing LLMs, it extracts insights, draws conclusions, and answers inquiries based on the provided data. The outcome is a comprehensive set of responses that thoroughly address the user's intent.

Concurrent multi-step inference feeds into the aggregation stage, enabling consistency checks like self-consistency. Additionally, industry-specific decoding strategies, such as speculative decoding, are applied for further refinement. This tailors the inference process to the specific domain, enhancing the relevance and accuracy of generated responses.

The service also routes issues to the most suitable expert model based on the problem's nature. By simultaneously invoking multiple LLMs with varying specializations, it leverages their diversity to improve the effectiveness of question answering.

\subsubsection*{\textbf{Aggregating Service}}
The Aggregating Service plays a crucial role in transforming reasoning outputs into clear, user-focused responses. It organizes reasoning outcomes into structured answers that are tailored to the user's initial query. This involves logically arranging information, ensuring clarity and conciseness, and maintaining user engagement.

This is essentially a trade-off between accuracy, latency, and system computational overhead. More complex CoT methods typically lead to a significant increase in latency. To address this, we use a "Reasoning \& Aggregating" approach to reduce system latency while compensating for the loss in accuracy by increasing computational overhead (e.g., by raising concurrency). This is an effective trade-off strategy in online scenarios.

Furthermore, in merging concurrent inference results, the service seamlessly combines outcomes from various inference processes, ensuring coherence and consistency. Techniques like self-consistency~\cite{wang2022self} are employed to validate and harmonize the aggregated results.

For industry-specific optimizations, the Aggregating Service incorporates several key elements:

\begin{itemize}
\item Citation and Transparency: Credibility is enhanced by incorporating citations~\cite{li2024citation} to reliable sources within industry contexts. This may involve referencing established sources and providing transparency about data origins. Additionally, the reasoning process, including the Chain of Thought and decision-making steps, can be showcased to offer deeper insights.

\item Tailored Formatting: Readability and visual appeal are improved by applying industry-standard formatting techniques, such as Markdown. Adhering to these conventions ensures consistency with established norms, making the content easier to understand.

\item Content Safety Integration: In safety-critical settings, content safety checks are integrated to filter out potentially harmful or inappropriate content. Algorithms and protocols are implemented to screen aggregated information, ensuring compliance with industry safety standards and regulations.
\end{itemize}

By integrating these components, the Aggregating Service does more than just consolidate reasoning results; it enhances the quality, trustworthiness, and safety of the final user response, ultimately delivering a smooth and enriching user experience.
